# Supplementary material for: On Practical Reinforcement Learning: Provable Robustness, Scalability, and Statistical Efficiency
Source: arXiv:2203.01758 source file (2022-03-03)
Supplement: Supplementary file 2 [file appendixC.tex]

% \section{Additional experiments}
% \label{chap3_section:additional_experiment}
